# Supplementary material for: VIRES: Video Instance Repainting via Sketch and Text Guided Generation
Source: arXiv:2411.16199 source file (2025-04-08)
Supplement: Supplementary file 1 [file 8_supplementary.tex]

\clearpage
\setcounter{page}{1}
\maketitlesupplementary

\subsection{Visualization of dataset}
% 展示结果说明图像分布差异很大，做跨域图像着色是具有挑战性的。out of distribution 的测试数据更加困难。
% 我们在第三章介绍了我们收集的跨域图像数据集。为了能更清楚的说明跨域图像的显著分布差异，我们展示了更多的数据样本。这些例子展示出跨域图像在纹理和内容上具有显著差距，表明论文跨域上色任务是具有挑战性的。
% 因此使用语言描述作为联系域鸿沟是非常重要的
%Sec.~\textcolor{red}{4.3.2}
In Sec.~\textcolor{red}{3}, we introduce the collected cross-domain colorization dataset. To elucidate the pronounced distributional disparities of cross-domain images more clearly, we present more data samples in \cref{fig:dataset}. These images exhibit significant variances in texture and content across different domains, thereby illustrating the challenging nature of our task in domain-adaptive colorization. It is further complicated when dealing with test data that are out of distribution. Consequently, the use of language descriptions to bridge domain gaps is of great importance.
% We present images and corresponding descriptions from our dataset. As shown in \cref{fig:dataset}, we demonstrate significant variations in data distributions, underscoring the challenging nature of cross-domain image colorization. 

% 

\subsection{Visualization of local color distribution map}
% 在第4章中，我们将减小局部颜色分布图的预测误差作为一个新的优化目标，以促进语言描述中的颜色在不同域的着色结果中被正确的表现出来。
% 在构建局部颜色分布图时，我们首先将像素的取值范围[0,255]分成了8个bin, 然后我们计算每个像素的值与它所属的bin中心点的距离，再除以bin的长度作为其属于该bin的概率。再使用第4章中提到的双边grid将其放缩到32*32分辨率。
%我们在图1中可视化红色通道的局部颜色分布图，可视化结果证明了它是一个域无关的颜色表示，不受纹理等的影响，因此可以作为一个跨域的颜色表示，增强着色模型的泛化性。
In Sec.~\textcolor{red}{4.3}, we introduce a novel optimization objective to minimize the prediction error of local color distribution maps \cite{lcd}. This approach aims to ensure that colors described in captions are accurately represented in the colorization results across different domains. To construct these local color distribution maps, we first divide the pixel value range $[0, 255]$ into 8 bins. We then calculate the distance of each pixel's value from the center of its corresponding bin, normalizing this distance by the bin length to determine the pixel's probability of belonging to that bin. Subsequently, using the bilateral grid \cite{realtimeei} illustrated in Sec.~\textcolor{red}{4.3}, we resize these maps to a $32\times 32$ resolution. In \cref{fig:lcd}, we visualize the local color distribution map for the red channel, demonstrating that it is a domain-independent color representation unaffected by factors such as texture. Hence, it can serve as a cross-domain color representation, enhancing the generalization capabilities of our colorization model.

% \subsection{Comparison with zero-shot diffusion}

\subsection{Additional comparison results}
% 我们展示更多与自然灰度图上色方法以及线稿上色方法的定性对比，以证明我们的模型在多个域上都能够与针对单一域的方法竞争甚至超过他们。
% 
We present an extensive qualitative comparison of our model with the methods for colorizing natural grayscale images (\eg, DDcolor \cite{ddcolor}, Color2Embedd \cite{color2embed}, and L-CoIns \cite{lcoins}), line arts (\eg, AlacGAN \cite{alacgan} and SGA \cite{sga}) and L-CAD \cite{lcad} as Sec.~\textcolor{red}{4.3}. As shown in \cref{fig:comp_gray} and \cref{fig:comp_sketch}, this comparison demonstrates that our model is capable of competing with, and in some cases surpassing, methods designed for single-domain applications.

\subsection{Additional ablation results}
We present more ablation results in \cref{fig:ablation} to study the impact of our proposed modules. The ablation details are described in Sec. \textcolor{red}{5.3} of the main paper.

\subsection{Failure case}
% 我们展示我们方法的failure case。 第一，我们的模型在给小物体上色时，容易出现颜色外溢的现象。这是由于在训练过程中输入图像的尺寸为256*256，这会使小物体细节丢失，特征提取困难，降低了定位小物体区域的准确性。第二，我们模型在给线稿上色时，由于部分线条的缺失会导致上色结果细节退化
We present failure cases of our method in \cref{fig:fail} to provide a comprehensive understanding of its limitations. First, our model tends to exhibit color bleeding when colorizing small objects. This issue stems from the training process, where input images are resized to $256 \times 256$ pixels, leading to the loss of fine details in small objects. Second, our model struggles with colorizing line art when some lines are missing. This absence of lines can result in a degradation of detail in the colorization results.

\subsection{Comparison with zero-shot diffusion}
